# Supplementary material for: Ion exchange gels enhance organic electrochemical transistor performance in aqueous solution
Source: arXiv:1909.13397 ancillary file (2019-09-29)
Supplement: Supplementary file 1 [file Bischak_Supplementary_Information_Ion_Exchange_Gels.pdf]

# Supplementary Information for

# Ion exchange gels for enhanced organic electrochemical transistor sensitivity and speed

Connor G. Bischak†, Lucas Q. Flagg†, David S. Ginger†*

†Department of Chemistry, University of Washington, Seattle, Washington 98195-1700, United States

**This PDF file includes:**

Materials and Methods

Supplementary Figures S1 to S7

Supplementary Movie Captions S1 to S4

Supplementary References

**Other Supplementary Materials for this manuscript include the following:**

Movies S1 to S4

**Materials and Methods**

Ion exchange gel fabrication

Poly(vinylidene fluoride-co-hexafluoropropylene) (PVDF-HFP) (Aldrich) was dissolved in N,N-dimethylformamide (DMF) at 50 mg/ml and stirred at 50 °C until the PVDF-HFP was dissolved completely. 1-Butyl-3-methylimidazolium bis(trifluoromethylsulfonyl)imide (BMIM TFSI) (Aldrich) was added to the solution in a 3:1 BMIM TFSI:PVDF-HFP ratio by weight and the solution was stirred at room temperature for 1 hr. The solution was then placed in a vacuum oven overnight at 90 °C until the DMF evaporated completely. The resulting ion gel was cooled at room temperature before use and had a thickness of 500 µm to 1 mm.

Organic electrochemical transistor (OECT) fabrication and measurement

OECT substrates were purchased from Nano Terra Inc. and were comprised of lithographically-patterned gold on polyethyelene terephthalate (PET) with transistor lengths of 20 µm and widths ranging from 50 to 2000 µm. Poly(3-hexylthiophene-2,5-diyl) (P3HT) (Ossila, M106) was dissolved in chlorobenzene (CB) (Aldrich) overnight at 50 °C at 20 mg/ml and spin-coated on the OECT substrate (thickness 80-150 nm). Poly[2,5-bis(3-tetradecylthiophen-2-yl)thieno[3,2-b]thiophene] (PBTTT, C14) (1-Material) was dissolved in 1,2-dichlorobenzene (DCB) (Aldrich) overnight at 20 mg/ml. Prior to spin-coating, the solution was heated to 80 °C and hot cast at 80 °C (thickness 30-80 nm). After spin coating, polymer was removed from all regions except for at the electrode junctions. The polymer-coated electrodes were then annealed at 160 °C under nitrogen. The exposed electrodes were then covered with an insulating layer of nitrocellulose (Sally Hansen, Insta-Dri Top Coat). Devices with and without the ion exchange gel were measured in degassed 100 mM KCl. Transfer curves were recorded by sweeping $V_G$ from -0.7 to 0 V vs Ag/AgCl and a fixed $V_{DS}$ of -0.6 V using two Keithley 2400 source measure units and custom Labview code. The step size was 0.01 V with 20 s between steps for both P3HT and PBTTT devices. Output curves were recorded at the same rate and step size for $V_G$ = -0.2 to -0.7 V for $V_{DS}$ = 0 to -0.7 V. For devices with the ion exchange gel, a 5 µL droplet of BMIM TFSI ionic liquid was pipetted onto the active layer to promote adhesion and the ion exchange gel was positioned above. Frequency-dependent transconductance measurements were performed using custom Matlab code with a Keithley 2400 source measure unit to apply $V_{DS}$ and an Agilent 33210A 10 MHz Function/Arbitrary Waveform Generator to modulate $V_G$. Both $V_G$ and $I_{DS}$ were recorded using a NI USB-6211 data acquisition card (National Instruments) with $I_{DS}$ measured as a voltage using a 200 Ω current shunt resistor and converted to current using Ohm's law. OECT switching speeds were measured in the same configuration with $V_{DS}$ = -0.6 and $V_G$ modulated between 0 V and -0.7 V with the Agilent waveform generator.

Spectroelectrochemistry ion injection kinetics measurements and cyclic voltammetry (CV)

Poly({4,8-bis[(2-ethylhexyl)oxy]benzo[1,2-b:4,5-b′]dithiophene-2,6-diyl}{3-fluoro-2-[(2-ethylhexyl)carbonyl]thieno[3,4-b]thiophenediyl}) (PTB7) and Poly[N-9′-heptadecanyl-2,7-carbazole-alt-5,5-(4′,7′-di-2-thienyl-2′,1′,3′-benzothiadiazole)], Poly[2,6-(4,4-bis-(2-ethylhexyl)-4H-cyclopenta [2,1-b;3,4-b′]dithiophene)-alt-4,7(2,1,3-benzothiadiazole)] (PCPDTBT) were purchased from Aldrich. For all spectroelectrochemistry measurements, the conjugated polymer was spin-coated on fluoride doped tin oxide (FTO) coated glass (Aldrich) or iodide doped tin oxide (ITO) coated PET from a 20 mg/ml solution in CB at room temperature (except for PBTTT, which was hot cast from dichlorobenzene (DCB, Aldrich) at 80 °C). Ion injection kinetics were measured with a MetroOhm Autolab PGSTAT204 with NOVA Software (version 2.1) and an Agilent 8453 spectrometer. The substrate served as the working electrode and was submerged in a cuvette containing degassed 100 mM KCl. An Ag/AgCl electrode (eDAQ) was used as the reference electrode and a Pt wire (Aldrich) was used as the counter electrode. UV-Vis measurements were collected with an integration time of 0.1 s/spectrum as the film was electrochemically doped. CVs were performed with a scan rate of 100 ms/step for 0.01 V steps. The current was integrated as a function of time to determine the charge as a function of time for stability measurements. For images and movies of the polymer partially covered by the ion exchange gel, a Microsoft Lumia 640 Smartphone was used to capture a movie either during a CV scan or after a 0.7 V bias was applied.

Ionic liquid-dependent doping measurements.

Trihexyltetradecylphosphonium chloride (THTDP Cl), THTDP bis(trifluoromethylsulfonyl)amide (TFSI), and THTDP dicyanamide (DCA) were purchased from Sigma Aldrich. The conjugated polymer (PBTTT or P3HT) was spin coated on the FTO coated glass as described in the previous section. Electrochemical measurements were performed as described in the previous section. Prior to inserting the polymer-coated FTO glass in the electrochemical cell, ~2 µL droplets of each ionic liquid were deposited. A bias was applied in 0.1 V steps in a range of 0 to 0.7 V (vs. Ag/AgCl) for 1 min/step, after which a photograph was taken using a Microsoft Lumia 640 Smartphone. Images were converted to greyscale for measuring the transparency underneath the droplet versus in regions directly exposed to the 100 mM KCl aqueous electrolyte.

Venus flytrap action potential measurements

Venus flytraps (*Dionaea muscipula*) were purchased from the Indoor Sun Shoppe (Seattle, WA). The gate electrode was comprised of a Ag wire wrapped around a wooden dowel that was placed in the soil adjacent to the plant. An OECT and standard Ag/AgCl wire electrode (A-M Systems) were placed adjacently on the same leaf. A Tektronix TDS 2024C Oscilloscope was used to record the voltage across the Ag/AgCl

standard electrode without additional amplification and two Keithley source measure units were used to apply the gate voltage ($V_G$) and the source-drain voltage ($V_{DS}$) and record changes in the source-drain current ($I_{DS}$). Signals were recorded from both electrodes while stimulating trigger hairs on the Venus flytrap leaf for OECTs with and without the ion exchange gel. For the series of action potentials, a small window was created in the flytrap leaf after the leaf closed. Action potentials were triggered by stimulating a trigger hair through this window to prevent any changes in contact between the OECT and the plant during the measurement.

## Supplementary Figures

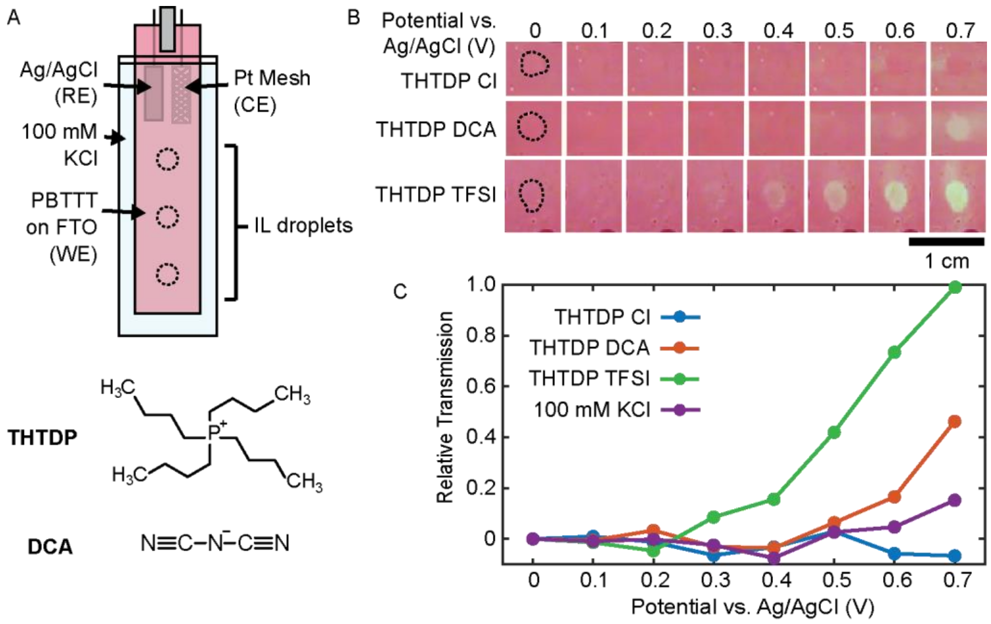


**Figure S1:** Ionic liquid-dependence of electrochemical doping of PBTTT. (A) Schematic of the experiment with multiple ionic liquid droplets deposited on the PBTTT film in an electrochemical cell and structure of the ionic liquid cation THTDP and anion DCA. (C) Extent of doping as a function of applied bias for three different ionic liquids and for 100 mM KCl. The trend closely matches that observed with different anions in an aqueous electrolyte.[1]

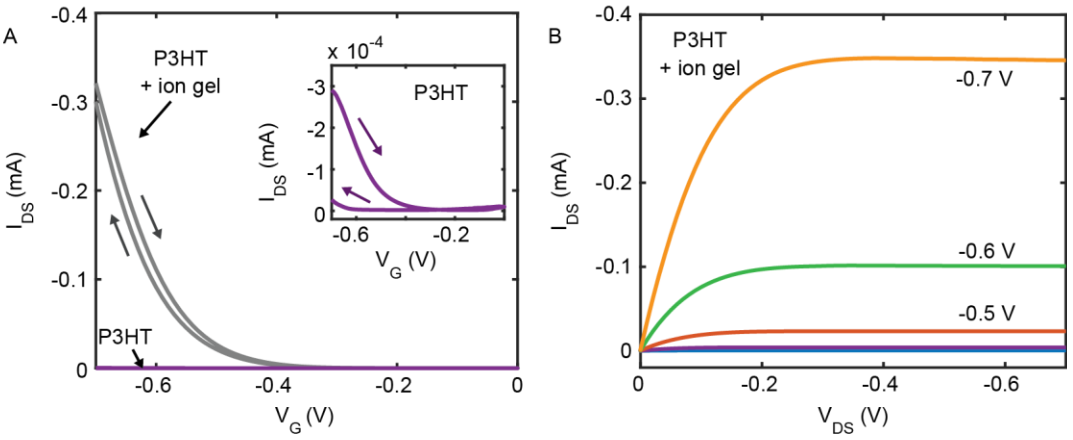


**Figure S2:** P3HT transistor data. (A) Example transfer curves for the same device before and after applying the ion exchange gel ($V_{DS}$ = -0.6 V, d = 110 nm, L = 20 $\mu$m, W = 100 $\mu$m). (B) Output curves recorded with the same device with the ion exchange gel present.

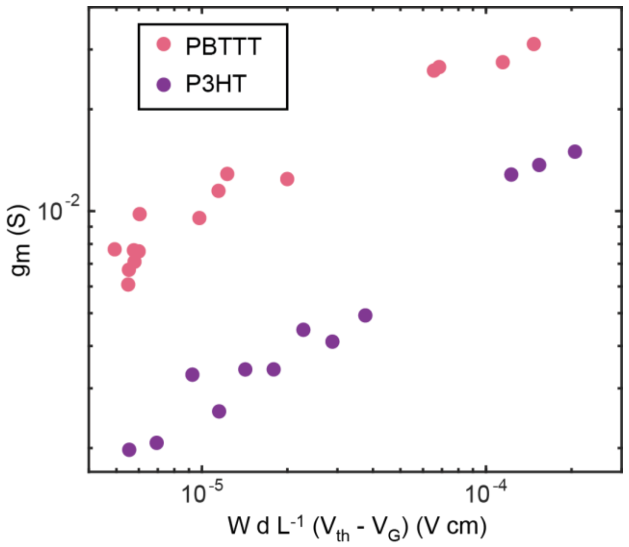


**Figure S3:** $\mu C^*$ plots of PBTTT (pink) and P3HT (purple) with the ion exchange gel applied.

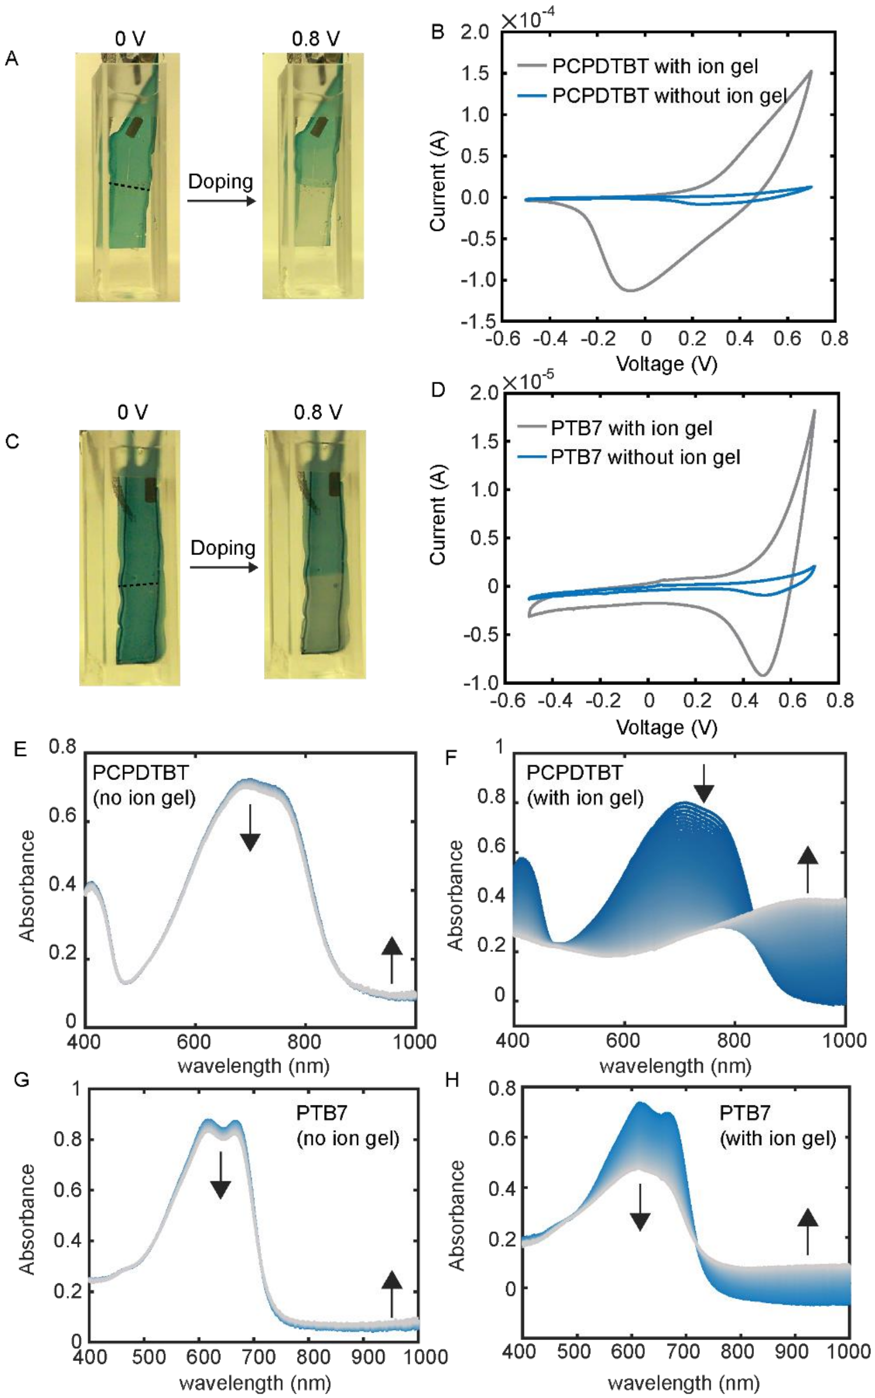


**Figure S4:** Ion exchange gel enhances doping in other hydrophobic polymers. PTB7 and PCPDTBT. (A) Image of PCPDTBT in an electrochemical cell with the ion gel applied before and after applying a 0.8 V bias (vs Ag/AgCl). (B) Cyclic voltammograms of PCPDTBT with and without the ion gel applied in 100 mM KCl. (C) Image of PTB7 in an electrochemical cell with the ion gel applied before and after applying a 0.8 V bias (vs Ag/AgCl). (D) Cyclic voltammograms of PTB7 with and without the ion gel applied in 100 mM KCl. Spectroelectrochemistry UV-Vis absorption spectra upon applying a 0.8 V bias for (E) PCPDTBT without the ion gel (F) PCPDTBT with the ion gel (G) PTB7 without the ion gel (H) PTB7 with the ion gel. The dotted lines in A and C show the edge of the ion exchange gel.

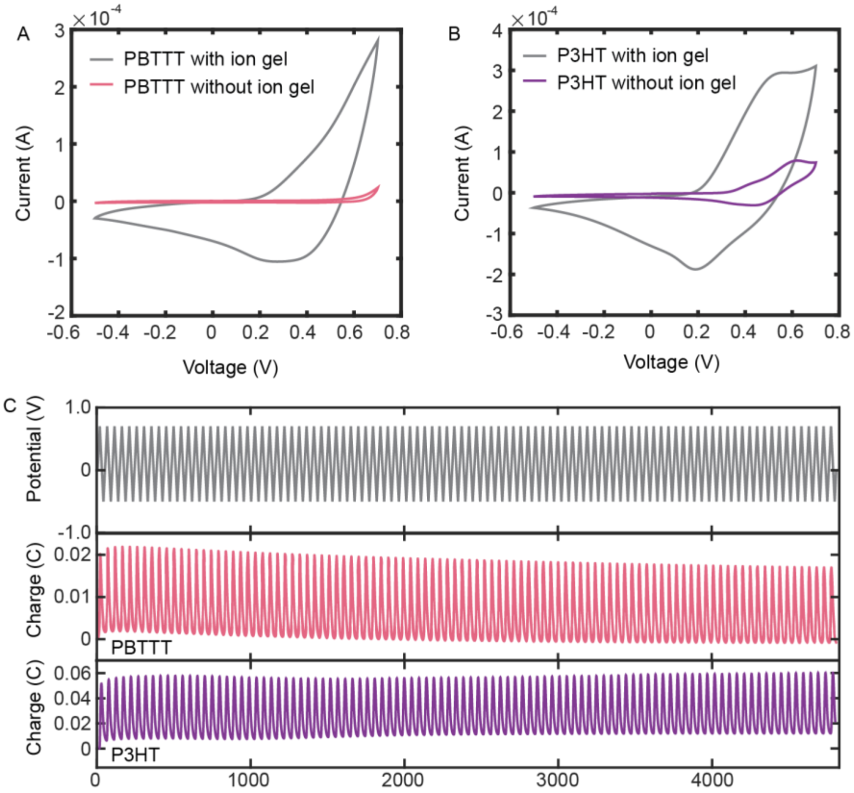


**Figure S5:** Stability of ion exchange gel OECTs upon repeated cycling. (A) Cyclic voltammograms of PBTTT with and without the ion gel. (B) Cyclic voltammograms of P3HT with and without the ion gel. (C) Charge accumulated in PBTTT and P3HT upon repeated cyclic voltammetry.

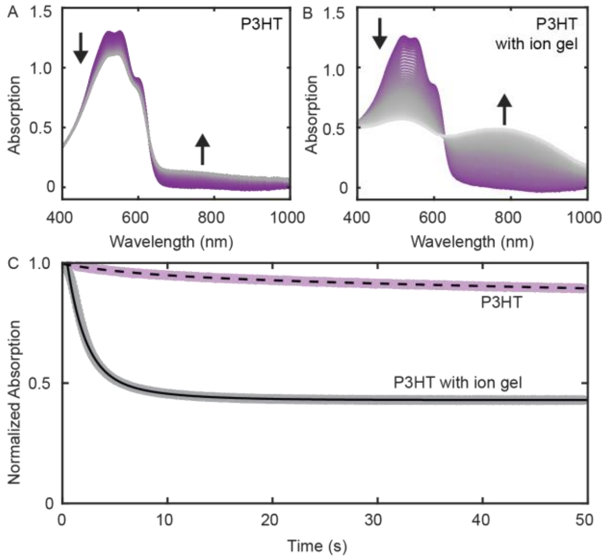


**Figure S6:** UV-Vis kinetics of P3HT. (A) Absorption spectrum as a function of time upon applying 0.7 V (vs. Ag/AgCl) in 100 mM KCl with 100 ms between spectra. (B) Absorption spectrum as a function of time upon applying 0.7 V (vs. Ag/AgCl) in 100 mM KCl with the ion exchange gel with 100 ms between spectra. (C) Peak absorption as a function of time for P3HT in 100 mM KCl and P3HT with the ion gel in 100 mM KCl.

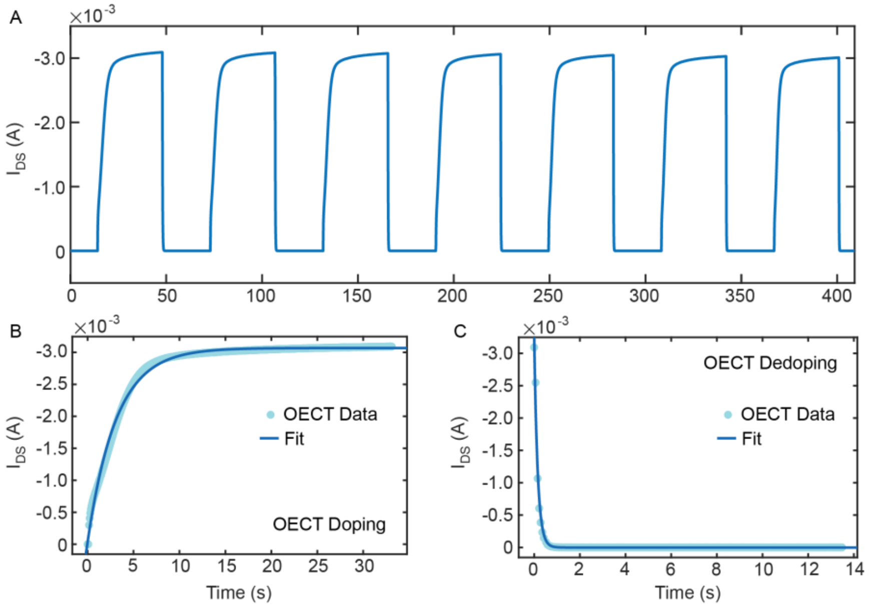


**Figure S7:** PBTTT with ion exchange gel transistor switching speeds. (A) Switching the transistor ON and OFF repeatedly from $V_G$ = 0 V to $V_G$ = -0.7 V at constant $V_{DS}$ = -0.6 V. (B) Fit of OECT $I_{DS}$ versus time during turn on with a single exponential. The characteristic ON time from the exponential fit is 3.1 ± 0.1 s. (C) Fit of OECT $I_{DS}$ versus time during dedoping with a single exponential. The characteristic OFF time from the exponential fit is 0.14 ± 0.01 s.

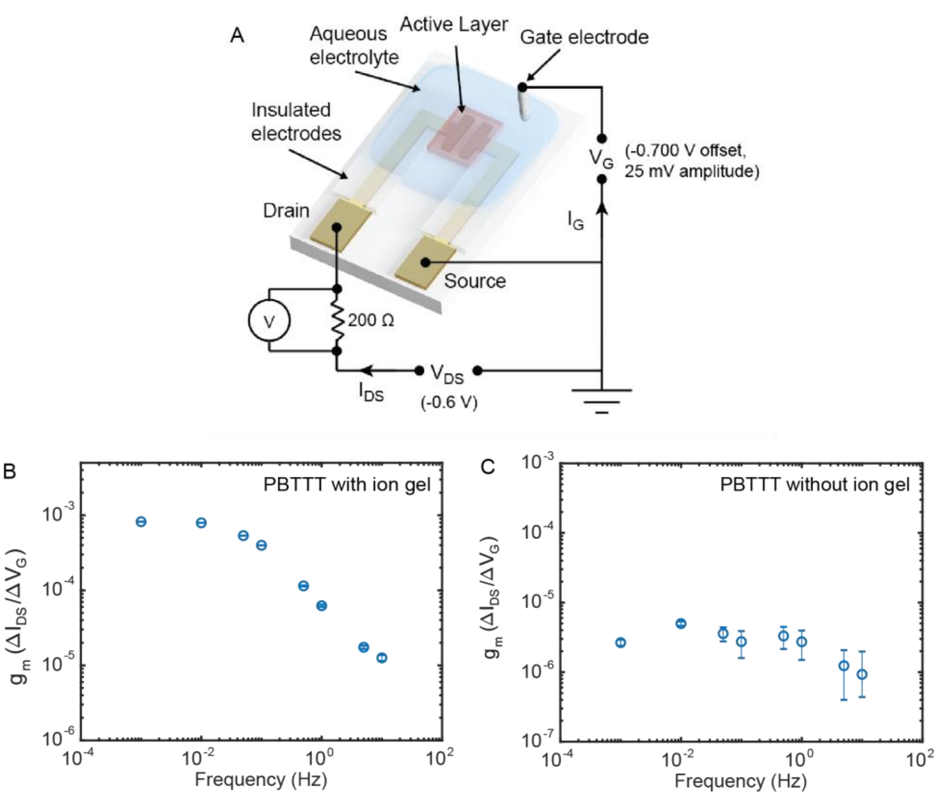


**Figure S8:** Frequency response of PBTTT OECTs with and without the ion exchange gel. (A) Schematic of the gain-bandwidth measurement. Transconductance as a function of frequency for a PBTTT OECT ($V_{DS}$ = -0.6 V, d = 55 nm, L = 20 $\mu$m, W = 1000 $\mu$m) (B) with and (C) without the ion exchange gel.

## Supplementary Movie Captions

**Movie S1:** Repeatedly cycling of PBTTT (-0.5 to 0.7 V vs Ag/AgCl) with an ion exchange gel applied in 100 mM KCl.

**Movie S2:** Repeatedly cycling of P3HT (-0.5 to 0.7 V vs Ag/AgCl) with an ion exchange gel applied in 100 mM KCl.

**Movie S3:** A single Venus flytrap action potential recorded with an ion exchange gel OECT showing that the trap does not close upon firing one potential.

**Movie S4:** Two Venus flytrap action potentials recorded with an ion exchange gel OECT showing the trap closing.

## Supplementary References


1. Flagg, L. Q., Giridharagopal, R., Guo, J. & Ginger, D. S. Anion-Dependent Doping and Charge Transport in Organic Electrochemical Transistors. *Chem. Mater.* **30**, 5380–5389 (2018).
